# Supplementary material for: SpatialToM: Modeling Multi-Agent Theory of Mind for Embodied Spatial Intelligence
Source: arXiv:2611.36849 source file (2026-12-02)
Supplement: Supplementary file 1 [file supp_contents.tex]

\makeatletter
\let\SpatialToMSavedAddtocontents\addtocontents
\renewcommand{\addtocontents}[2]{%
  \def\SpatialToMContentsStream{#1}%
  \def\SpatialToMMainContentsStream{toc}%
  \ifx\SpatialToMContentsStream\SpatialToMMainContentsStream
    \SpatialToMSavedAddtocontents{stoc}{#2}%
  \else
    \SpatialToMSavedAddtocontents{#1}{#2}%
  \fi
}
\makeatother

\onecolumn
\begingroup
\ifdefined\nolinenumbers\nolinenumbers\fi
\begin{center}
  {\large\bfseries\thetitle\par}
  \vspace{0.4em}
  {\large Supplementary Material\par}
\end{center}
\vspace{0.4em}
\hypersetup{linkcolor=black,linktoc=all}
\fontsize{10}{11}\selectfont
\makeatletter
\c@tocdepth=2\relax
\patchcmd{\l@section}{1.0em}{0.45em}{}{}%
\let\SpatialToMSavedStarttoc\@starttoc
\renewcommand{\@starttoc}[1]{\SpatialToMSavedStarttoc{stoc}}
\let\SpatialToMSavedContentsline\contentsline
\renewcommand{\contentsline}[4]{%
  \def\SpatialToMContentsTitle{#2}%
  \patchcmd{\SpatialToMContentsTitle}{\hskip -1em.\nobreakspace {}}{}{}{}%
  \SpatialToMSavedContentsline{#1}{\SpatialToMContentsTitle}{#3}{#4}%
}
\makeatother
\tableofcontents
\clearpage
\endgroup
\twocolumn
